# Supplementary material for: Cosmos: Compressed and Smooth Latent Space for Text Diffusion Modeling
Source: arXiv:2506.21170 source file (2026-01-05)
Supplement: Supplementary file 1 [file ablation_wikipedia.tex]

\subsection{Empirical analysis of autoencoder training regimes on Wikipedia dataset}
\label{app:ablation_wikipedia}

\begin{wraptable}{r}{0.5\textwidth}
%\renewcommand{\arraystretch}{0.5}
%\vspace{-4mm}
\centering
\caption{Comparison of autoencoder training regimes on text generation quality on \textsc{Wikipedia}. Features are added cumulatively from top to bottom.}
\label{tab:wiki:training-ablation}

% Define a light gray background color for best rows
\definecolor{bestrow}{gray}{0.85}

\begin{tabular}{@{}lccc@{}}
\toprule
\textbf{Configuration}             & \textbf{MAUVE}~$\uparrow$ & \textbf{PPL}~$\downarrow$ & \textbf{Div}~$\uparrow$ \\
\midrule
\textbf{CE($\bf{w, \hat{w}}$)}                                & $0.056$ & $385.6$ & $0.590$ \\
\midrule
 \textbf{+ MSE($\bf{h, \hat{h}}$)}          & $0.069$ & $344.4$ & $0.625$ \\
\midrule
\multicolumn{4}{l}{\textbf{+ Random masking (rate)}}                              \\
 \quad 0.3                                 & $0.081$ & $289.1$ & $0.594$ \\

\midrule
\multicolumn{4}{l}{\textbf{+ Gaussian noising ($\delta$)}}                       \\
\quad 0.7                                 & $0.103$ & $205.0$ & $0.588$ \\
\midrule
\multicolumn{4}{l}{\textbf{+ Latent dropout (rate)}}                             \\
\quad 0.4                                 & $0.112$ & $186.7$ & $0.581$ \\
\bottomrule
\end{tabular}
\vspace{-5mm}
\end{wraptable}

We also conduct a large-scale ablation on the \textsc{Wikipedia} dataset with $N = 16$ latents and max sequence length $L=128$, following a setup analogous to that in \cref{sec:exp:ablation}. Results, presented in Table~\ref{tab:wiki:training-ablation}, reveal trends consistent with those observed in the small-scale ablation. Notably, applying the proposed training modifications leads to substantial improvements in evaluation metrics. The final model approaches the performance of the TEncDM baseline \cite{shabalin2025tencdm}, while operating in a latent space that is $8 \times$ smaller.

Additionally, we investigate how scaling the latent space length on \textsc{Wikipedia} affects performance. We experiment with latent sequence lengths ranging from $16$ to $128$. As expected, we observe steady performance improvements with longer latent sequences. Results are provided in \Cref{tab:latent-length-scaling}.

\begin{table}[h] % {0.4\textwidth}
  % \vspace{-1em}
  
  \setlength{\tabcolsep}{10pt}
  \caption{Impact of scaling the number of latent vectors $N$ on unconditional generation quality on \textsc{Wikipedia}.}
  \label{tab:latent-length-scaling}
  \centering
  % \small
  \begin{tabular}{@{}lccc@{}}
    \toprule
    \textbf{$N$} & \textbf{MAUVE} $\uparrow$ & \textbf{PPL} $\downarrow$ & \textbf{Div} $\uparrow$ \\
    \midrule
     Source  & 0.953 & 21.7 & 0.403 \\
    \midrule
    BERT repr.  & 0.109 & 173.1 & 0.562 \\ 
    \midrule
    16   & 0.112 & 186.7  & 0.581 \\
    32   & 0.149 & 134.4  & 0.579 \\
    64   & 0.157 & 128.1 & 0.582 \\
   128   & 0.173 & 118.2  & 0.592 \\
    \bottomrule
  \end{tabular}
  % \vspace{-1em}
\end{table}
